# Supplementary material for: threaTrace: Detecting and Tracing Host-based Threats in Node Level Through Provenance Graph Learning
Source: arXiv:2111.04333 source file (2021-11-08)
Supplement: Supplementary file 1 [file appendix.tex]

\appendices

\section{Some Details of threaTrace}

\label{section:a1}

In this section, we provide some supplementary details of GraphSAGE's concept, \textsc{threaTrace}'s executing procedure, and \textsc{threaTrace}'s feature extraction method.

\begin{algorithm}[t]
\caption{Forward propagation (FP) of GraphSAGE}
\label{alg:4}
\LinesNumbered
\KwIn{Graph $G = (V, E, \mathcal{X}_v, \mathcal{X}_e, \mathcal{T}_e)$; features assigning function $\mathcal{F} : V \rightarrow \mathbb{N}^{2*N_e}$; hop number $K$; neighborhood function $\mathcal{N} : V \rightarrow 2^V$; a set of weight matrices $\mathbf{W}^k, \forall k \in \{1, ..., K\}$; aggregator functions ${AGGREGATE}_k, \forall k \in \{1, ..., K\}$; nonlinear activation function $\sigma$)}
\KwOut{vector representations $z_v$ for $\forall v \in V$}
$t_v^0 \leftarrow \mathcal{F}(v), \forall v \in V$\;
\For{$k = 1 ... K$}{
	\For{$v \in V$}{
$t_{\mathcal{N}(v)}^k \leftarrow AGGREGATE_k(\{t_u^{k-1},\forall u \in \mathcal{N}(v)\})$\;
$t_v^k \leftarrow \sigma(\mathbf{W}^k \cdot \text{CONCAT}(t_v^{k-1}, t_{\mathcal{N}(v)}^k))$ \;
	}
$t_v^k \leftarrow t_v^k / \Arrowvert t_v^k \Arrowvert_2 , \forall v \in V $\;
}

\end{algorithm}

\subsection{GraphSAGE concept}
\label{section:a1.1}

GraphSAGE is the base model of \textsc{threaTrace}. We introduce the concept and algorithm of GraphSAGE in this subsection. GraphSAGE is an inductive GNN method. Like other traditional deep learning algorithms, it uses forward propagation to compute the embedding of a node and use backward propagation to optimize the parameters of the model. The forward propagation algorithm first takes a graph $G = (V, E)$ as input, and then iteratively computes the embedding of each node. The embedding procedure is shown in Algorithm \ref{alg:4}. Once the embedding of a node is calculated, GraphSAGE computes its loss and then performs backward propagation to optimize the parameters of the model.

\textbf{Aggregator functions.} GraphSAGE utilizes aggregator functions to aggregate information from a node's neighbor as shown in Algorithm \ref{alg:4}. There are three candidate aggregator functions as follow:

\textbf{(1) Mean aggregator.} Mean aggregator simply takes the elementwise mean of the vectors in $\{t^{k-1}_u, \forall u \in \mathcal{N}(v)\}$.

\textbf{(2) LSTM aggregator.} It is a more complex aggregator based on an LSTM architecture \cite{70}. LSTM has better expressive capability compared to mean aggregator. LSTM is not permutation invariant because it processes the inputs sequentially. Therefore, LSTM aggregator takes a random permutation of the nodes' neighbors as input to operate in an unordered set.

\textbf{(3) Pooling aggregator.} Pooling aggregator is trainable. Each neighbor's features are fed through a fully-connected neural network independently. An elementwise max-pooling function is applied for neighbor's information aggregation:

\begin{equation}
\label{equa:5.7}
AGGREGATE^{pool}_k = max(\{\delta(W_{pool} t^k_{u_i}+b), \forall u_i \in \mathcal{N}(v)\})
\end{equation}

The aggregator that \textsc{threaTrace} uses is \textbf{Mean aggregator}. We choose mean aggregator because LSTM aggregator and pooling aggregator are more complex than mean aggregator, which will increase the computational expense.

\begin{algorithm}[t]
\caption{Feature extraction method}
\label{alg:4.3}
\LinesNumbered
\KwIn{Graph $G = (V, E, \mathcal{X}_v, \mathcal{X}_e, \mathcal{T}_e)$; num of different edge types $N_e$; Node type map function $\mathcal{M}_v : \sum \rightarrow \mathbb{N}$; Edge type map function $\mathcal{M}_e : \sum \rightarrow \mathbb{N}$; $In : V \rightarrow 2^E$; $Out : V \rightarrow 2^E$}
\KwOut{Label mapping function $\mathcal{L} : V \rightarrow \{0, ..., N_n\}$ and feature mapping function $\mathcal{F} : V \rightarrow \mathbb{N}^{2*N_e}$}

\For{$v \in V$}{
	$f \leftarrow \text{zeros}(2*N_e)$\;
\For {$e \in In(v)$} {
		$f[\mathcal{M}_e(\mathcal{X}_e(e))] \leftarrow f[\mathcal{M}_e(\mathcal{X}_e(e))] + 1$\;
	}
\For {$e \in Out(v)$} {
		$f[\mathcal{M}_e(\mathcal{X}_e(e)) + N_e] \leftarrow f[\mathcal{M}_e(\mathcal{X}_e(e)) + N_e] + 1$\;
	}
	$\mathcal{L}(v) \leftarrow \mathcal{M}_v( \mathcal{X}_v(v))$\;
	$\mathcal{F}(v) \leftarrow f$
}
\end{algorithm}

\begin{algorithm}[t]
\caption{Executing method of multi-model framework}
\label{alg:4.5}
\LinesNumbered
\KwIn{Subgraph $\hat{G} = (V, E, \mathcal{X}_v, \mathcal{X}_e, \mathcal{T}_e)$; nodes to be detected $\hat{V} \subset V $; features mapping function $\mathcal{F} : V \rightarrow \mathbb{N}^{2*N_e}$; Label mapping function $\mathcal{L} : V \rightarrow \{0, ..., N_n\}$; hop number $K$; submodels number $cnt$}
\KwOut{ abnormaly nodes $A \subset \hat{V}$}

\For {$k = 0 ... \text{cnt-1}$}{
	current submodel $\leftarrow \mathbb{M}_k$\;
	$z \leftarrow \text{FP}(\hat{G}, \mathcal{F}, K, AGGREGATE_k, \mathbf{W}^k, \sigma)$\;
	$\hat{z} \leftarrow z_{\forall v \in \hat{V}}$ \;
	$M \leftarrow \text{softmax}(\hat{z})$\;
	\For {$v \in \hat{V}$} {	
		$C_v \leftarrow$ index of the biggest element in $M_v$\;
		$\hat{C}_v \leftarrow$ index of the second biggest element in $M_v$\; 
		\If {$C_v = \mathcal{L}(v) \text{ and } M_{vC_v}/M_{v\hat{C_v}} > R'_t$} {
			remove $v$ from $\hat{V}$ \;
		}
	}
	$A \leftarrow \hat{V}$
}

\end{algorithm}

\subsection{Procedure of executing phase and feature extraction method}
\label{section:a1.2}

The executing method which may help understand the workflow of \textsc{threaTrace} is shown in Algorithm \ref{alg:4.5}. It demonstrates how the multi-model framework of \textsc{threaTrace} is used for anomalous nodes detection. Specifically, the multi-model framework takes a subgraph $\hat{G}$ and nodes set $\hat{V}$ to be detected as input, and iteratively detects $\hat{V}$ in the submodels. If a node is correctly classified in the current working submodel, it will be removed from $\hat{v}$ (line \textbf{6-12} in Algorithm \ref{alg:4.5}). After executing all submodels, the rest nodes in $\hat{v}$ are detected as anomalous nodes.

The feature extraction method is shown in Algorithm \ref{alg:4.3}. We set a node's label as its node type (line \textbf{9} in Algorithm \ref{alg:4.3}), and extract its features as the distribution of numbers of different edges' types related to it (line \textbf{2-8, 10} in Algorithm \ref{alg:4.3}).

\section{Adversarial Robustness}
\label{section:a2}

We study the optimization-based evasion attack detailedly in this section.

\begin{figure}[htbp]
\centerline{\includegraphics[width=0.3\textwidth]{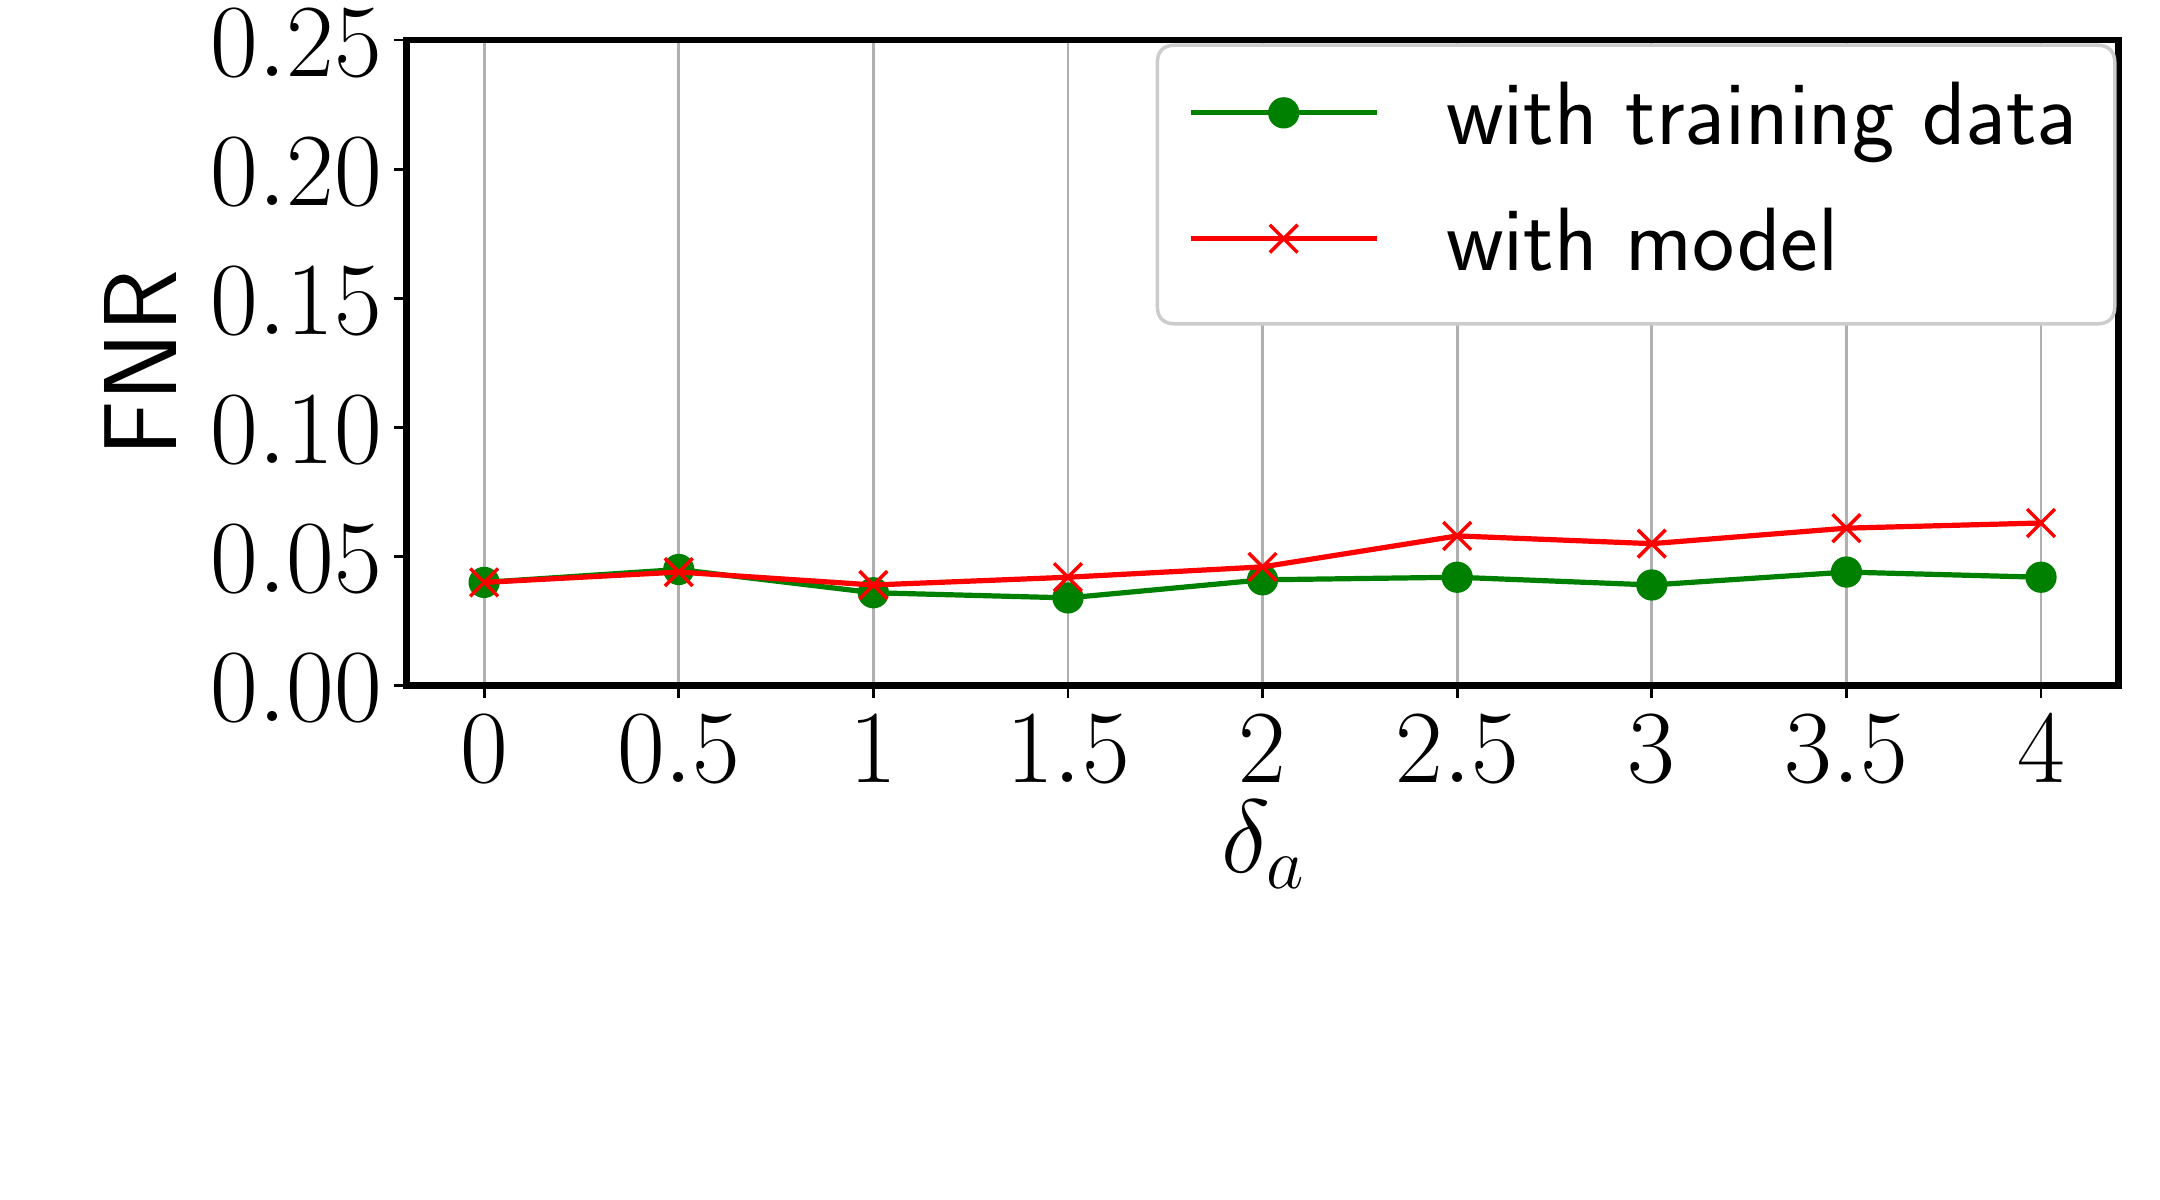}}
\caption{Result of optimization-based evasion attack experiments.}
\label{fig:11}
\end{figure}

\textbf{Attack Methodology.} \textsc{threaTrace} is a Graph-based detection system. Therefore, we borrow the idea of existing adversarial attack against Graph-based detectors \cite{67, 68, 69} to develop an adaptive attack on \textsc{threaTrace}, called optimization-based evasion attack. The purpose of this attack is to make abnormal nodes evade the detection of \textsc{threaTrace} in the execution phase. Specifically, because \textsc{threaTrace} judges the node as abnormal when it is misclassified, the purpose of the attacker is to make the abnormal node be classified into the correct class to avoid detection. In order to evade detection, the attacker can conduct perturbation in feature space or original space. The former method directly changes a sample's feature and changes the attacker's original behavior base on the new feature. The latter method directly changes the original behavior. Because \textsc{threaTrace}'s feature extraction method is not complex and perturbating the feature space is usually more effective than perturbating the original space, we study the feature space perturbation in this paper. The attacker needs to find a perturbation on the abnormal node's feature which is constructed with edges between the node and its neighbor. Note that we suppose the attacker has compromised the system by implanting some abnormal nodes (such as \textit{Malware}, \textit{Remote Shell}, anomalous \textit{Dynamic Link Library}) into it. Therefore, the attacker can control the related edges of the abnormal nodes. The perturbation should be as small as possible to keep the original function of the abnormal node and reduce cost. In a word, suppose $x$ is the feature of an abnormal node which can be detected by \textsc{threaTrace} originally, the optimization-based evasion attack's goal is to change the feature to $\hat{x}$ to evade detection with the constraint $\frac{\left\|\hat{x}-x\right\|_2}{\left\|x\right\|_2} < \delta_a$, where $\delta_a$ limits the perturbation. In order to construct a node's adversarial features $\hat{x}$, we assume that the attacker knows \textsc{threaTrace}'s feature extraction method mentioned in \S\ref{section:4}. For other adversarial's background knowledge of \textsc{threaTrace}, we study two kinds of attackers based on the background knowledge.

\textit{(1) Attackers with training data.} This kind of attacker does not know \textsc{threaTrace}'s model, but has the training data. The optimization-based evasion attack with this background knowledge can be performed in two steps. The first step is to find a benign node $x_b$ in the training data, which is most similar to the anomalous node $x$ and has the same class as $x$. Formally,

\begin{equation}
\label{equa:6}
argmin_{x_b} \left\|x_b-x\right\|_2 \quad s.t. \quad class(x_b) = class(x)
\end{equation}

The second step is to solve the optimization problem, which is not difficult:

\begin{equation}
\label{equa:7}
argmin_{\hat{x}}\left\|\hat{x}-x_b\right\|_2 \quad s.t. \quad \frac{\left\|\hat{x}-x\right\|_2}{\left\|x\right\|_2} < \delta_a, \hat{x} \in \mathbb{N}
\end{equation}

\textit{(2) Attackers with \textsc{threaTrace}'s model.} This kind of attacker knows \textsc{threaTrace}'s model, including the parameters after training and hyperparameters. Therefore, the attacker can solve the optimization problem directly based on the loss of the model. Formally,

\begin{equation}
\label{equa:8}
argmin_{\hat{x}}(loss(\hat{x})) \quad s.t. \quad \frac{\left\|\hat{x}-x\right\|_2}{\left\|x\right\|_2} < \delta_a, \hat{x} \in \mathbb{N}
\end{equation}

$Loss(\hat{x})$ is the loss function of \textsc{threaTrace}, indicating whether a sample is classified into the correct category. For an anomalous sample, the attacker needs to make \textsc{threaTrace} correctly classify it to evade detection. Therefore, $loss(\hat{x})$ should be as small as better. This problem can be easily solved by a gradient-based method. \textsc{threaTrace} consists of several submodels. For simplicity, we choose the first submodel for the target model to evasion.

For these two kinds of attackers, once $\hat{x}$ is successfully solved, the attacker controls the abnormal node to interact with other nodes in the system according to the new distribution of edges, so that its feature will change to $\hat{x}$.

\noindent\textbf{Robustness Evaluation and Analysis.} We use Unicorn SC-2 dataset for evaluation. We first choose the abnormal nodes detected by \textsc{threaTrace} as the base samples and then apply the optimization-based evasion approach to compute $\hat{x}$ for each abnormal node. After that, we change the related edges of the adversarial samples to change their features extracted. For attackers with training data, the experimental results are shown in Figure \ref{fig:11}. The results demonstrate that without grasping the model, only imitate the training data has almost no effect on evasion detection. For attackers with \textsc{threaTrace}'s model, the results demonstrate that with the increasing of $\delta_a$, the evasion effection also increases. However, compared to the original result, the FNR is acceptable (raise from 0.04 to 0.07), which demonstrates \textsc{threaTrace}'s good robustness against optimization-based evasion attack. We find that the features of some benign nodes will also be affected if the related edges of abnormal nodes are changed. Therefore, these benign nodes will be detected as abnormal, making the abnormal graph be alerted. Based on this discovery, we redesign the optimization function to consider benign neighbor nodes of the attack node, as shown follow.

\begin{equation}
\begin{split}
\label{equa:9}
argmin_{\hat{x}} loss(\hat{x})+\Sigma loss(x_i), x_i \in neighbor(\hat{x}) \\ 
s.t. \quad \frac{\left\|\hat{x}-x\right\|_2}{\left\|x\right\|_2} < \delta_a , \hat{x} \in \mathbb{N}
\end{split}
\end{equation}

We use the new function to generate adversarial samples and evaluate the evasion effect. The results (orange line in Figure \ref{fig:11}) show that the new function has a better evasion effect, but there is no essential difference from the old function. We think the reason is that there are three constraints in \ref{equa:9}, which make it difficult to get an ideal solution.

\begin{table}[b]
\setlength{\abovecaptionskip}{0.cm}
\setlength{\belowcaptionskip}{-0.3cm}
\centering

\caption{Overview of StreamSpot dataset.}
\label{table:1.5}
\scalebox{0.9}{
\begin{tabular}{|c|c|c|c|}
\hline
\textbf{Scene}&\textbf{\# of graph}&\textbf{Average \# of nodes}&\textbf{Average \# of edges} \\
\hline
\text{Benign} & \text{500} & \text{8315} & \text{173857}\\
\hline
\text{Attack} & \text{100} & \text{8891} & \text{28423}\\
\hline
\end{tabular}
}
\vspace{0mm}
\end{table}

\begin{table}[b]
\setlength{\abovecaptionskip}{0.cm}
\setlength{\belowcaptionskip}{-0.3cm}
\centering

\caption{Overview of Unicorn SC-2 dataset.}
\label{table:2.5}
\scalebox{0.9}{
\begin{tabular}{|c|c|c|c|}
\hline
\textbf{Scene}&\textbf{\# of graph}&\textbf{Average \# of nodes}&\textbf{Average \# of edges} \\
\hline
\text{Benign} & \text{125} & \text{238338} & \text{911153}\\
\hline
\text{Attack} & \text{25} & \text{243658} & \text{949887}\\
\hline

\end{tabular}
}
\vspace{0mm}
\end{table}

\begin{table}[b]
\setlength{\abovecaptionskip}{0.cm}
\setlength{\belowcaptionskip}{-0.3cm}
\centering
\caption{Overview of DARPA TC dataset.}
\label{table:4}
\scalebox{0.8}{
\begin{tabular}{|c|c|c|c|c|}
\hline
\textbf{Scene}&\textbf{System}&\textbf{\# of benign nodes}&\textbf{\# of abnormal nodes}&\textbf{\# of edges}\\
\hline
\text{THEIA} & \text{Ubuntu} & \text{3505326} & \text{25362} & \text{102929710}\\
\hline
\text{Trace} & \text{Ubuntu} & \text{2416007} & \text{67383} & \text{6978024}\\
\hline
\text{CADETS} & \text{FreeBSD} & \text{706966} & \text{12852} & \text{8663569}\\
\hline
\text{fivedirections} & \text{Windows} & \text{569848} & \text{425} & \text{9852465}\\
\hline
\end{tabular}
}
\vspace{0mm}
\end{table}

\section{Detailed Experimental Settings}
\label{section:a3}

In this section, we introduce details of the datasets we use, comparison work's implementations, experimental settings and evaluation metrics. Some content is introduced in \S\ref{section:6} and summarized here.

\subsection{Datasets}
\label{section:a3.0}

We use three public datasets for evaluation which are detailedly introduced below.

\noindent\textbf{StreamSpot dataset.} The StreamSpot dataset (Table \ref{table:1.5}) is StreamSpot's own dataset which is publicly available \cite{32}. It contains 6*100 information flow graphs derived from five benign scenes and one attack scene. Each scene runs 100 times to generate 100 graphs using the Linux SystemTap logging system \cite{64}. The benign scenes involve different benign activities: checking Gmail, browsing CNN.com, downloading files, watching YouTube, and playing a video game. The attack scene involves a drive-by download attack. The victim host visits a malicious URL, which exploits a Flash vulnerability and gets root access to the victim.

\noindent\textbf{Unicorn SC-2 dataset.} This dataset is Unicorn's own dataset \cite{49}, which is more complex than the StreamSpot dataset. The Unicorn SC-2 dataset (Table \ref{table:2.5}) is generated in a controlled testbed environment following the typical cyber kill chain model. Each graph, which is captured by CamFlow (v0.5.0), contains the whole-system provenance of a host running for three days. There are background benign activities in both benign and attack graphs. For attack graphs, the attacker exploits a vulnerability (CVE-2014-6271) from GNU Bash version 4.3 to execute arbitrary code remotely via crafted trailing strings after function definitions in Bash scripts.

\noindent\textbf{DARPA TC dataset.} DARPA TC dataset (Table \ref{table:4}) is generated in the third red-team vs. blue-team engagement of the DARPA Transparent Computing program. The engagement lasted for two weeks and the provenance data and ground truth are publicly available \cite{47}. During the engagement, the red team performed attacks and benign background activity on hosts with different systems. Three kinds of attackers are involved in the red-team, including Nation State, CommonThreat, and Metasploit. The Nation State attackers' goal is to steal proprietary and personal information from the targeted company. They use the Nginx backdoor, the Firefox backdoor, the browser extension, Drakon APT, and micro APT to accomplish the goal. The Common Threat attackers' goal is to steal personally identifiable information for financial gain by deceiving the targeted users into providing access to the target network. They accomplish the goal using phishing e-mails, PowerShell scripts, a malicious Excel spreadsheet macro, a Pine backdoor, and a malware executable. The Metasploit attackers try and fail to perform the attack using EternalBlue. Provenance collecting tools in those systems captured provenance data of the whole system from start to end.

\subsection{Implementations}
\label{section:a3.1}

The implementation of \textsc{threaTrace} is introduced in \S\ref{section:5}. We compare \textsc{threaTrace} with three state-of-the-art anomaly-based threat detection systems (StreamSpot, Unicorn, and ProvDetector) in this paper. Thus, we introduce their implementations in this subsection. StreamSpot and Unicorn are open-sourced. We directly use the open-source implementations and run their projects to get the results. Unfortunately, ProvDetector is not open-sourced. Therefore, we reimplement it according to the methods proposed in the original paper. For StreamSpot and Unicorn, the results of the open source project are almost the same as the original papers (or better than the original papers). For ProvDetector, we cannot compare the performance with the original paper because we do not have the private dataset of the paper for evaluation. Note that there are some state-of-the-art misuse-based methods \cite{7,8,58,65}. We cannot reimplement them for evaluation because their rulesets are private, which are important for misuse-based methods.

\subsection{Experimental Settings}
\label{section:a3.2}

\noindent\textbf{Hardware.} Experiments of \textsc{threaTrace} and the comparison methods are all conducted in an Ubuntu 16.04.6 LTS machine with 16 vCPUs and 64GiB of memory

\noindent\textbf{Parameters of \textsc{threaTrace}}. The manually setted parameters of experiments in \S\ref{section:6.1}, \ref{section:6.2}, \ref{section:6.3}, \ref{section:a2}, \ref{section:a4}, \ref{section:a5} are shown in Table \ref{table:1}. Each submodel of \textsc{threaTrace} has the same GraphSAGE's hyperparameters. Specifically, we set most of those hyperparameters as default values and set the number of hidden layer's neurons as 32 and the number of hidden layer as 1.

\noindent\textbf{Settings of \S\ref{section:6.1}.} We evaluate and compare \textsc{threaTrace}'s graph-level threat detection performance with StreamSpot and Unicorn in \S\ref{section:6.1}. The dataset we used is StreamSpot dataset, which is StreamSpot's own dataset \cite{32}. An introduction of StreamSpot dataset is available in \S\ref{section:6.1}. Experiments are performed repeatedly in order to gain the mean results (same for other experiments). We randomly split the dataset into a training set with 75*5 benign graphs and a testing set with 25*5 benign graphs and 25 attack graphs. This validation strategy is the same as Unicorn. The results of Unicorn's open source project are almost the same as the original paper. The results in StreamSpot's origin paper lack some metrics (Recall, F-score, and FPR). Therefore, we use the open-source project and follow the same validation strategy to run StreamSpot. We set StreamSpot's parameters as the default values in the open-source project. The result is not exactly the same as the original paper. It is probably caused by the different validation strategies. We do not compare with ProvDetector because ProvDetector needs to analyze edges' timestamp, which is not included in StreamSpot dataset.

\noindent\textbf{Settings of \S\ref{section:6.2}.} We evaluate and compare \textsc{threaTrace}'s graph-level threat detection performance with Unicorn and ProvDetector in \S\ref{section:6.2}. The dataset we used is Unicorn SC-2 dataset, which is Unicorn's own dataset \cite{49}. An introduction of Unicorn SC-2 dataset is available in \S\ref{section:6.2}. We follow the same 5-fold cross-validation as Unicorn: use 4 groups (each group contains 25 graphs) of benign graphs to train, and the 5th group of benign graphs and 25 attack graphs for validation. A streaming mode is applied to replay the validation graphs and make detection dynamically. We do not compare with StreamSpot because StreamSpot cannot deal with a large number of edges \cite{19}.

\noindent\textbf{Settings of \S\ref{section:6.3}.} We evaluate \textsc{threaTrace}'s node-level threat detection performance and compare \textsc{threaTrace}'s graph-level threat detection performance with Unicorn and ProvDetector in \S\ref{section:6.3}. The dataset we used is DARPA TC dataset, which is generated in the third red-team vs. blue-team engagement of the DARPA Transparent Computing program. An introduction of DARPA TC dataset is available in \S\ref{section:6.3}. We first follow the groundtruth of the engagement to label nodes and split the graphs into benign training set and mixture testing set. The number of graphs in training set and testing set is 5*4 and 5*4. For graph-level experiments, we use the training set for training and evaluate \textsc{threaTrace}, Unicorn, and ProvDetector in the testing set. For node-level experiments, we evaluate \textsc{threaTrace} separately because the comparison methods do not have the ability of node-level detection. We cannot compare with misuse-based methods because we do not have the private ruleset.

\noindent\textbf{Settings of \S\ref{section:6.4}.} In \S\ref{section:6.4}, we evaluate \textsc{threaTrace}'s graph-level threat detection performance with varying parameters in Unicorn SC-2 dataset. The parameters we evaluate are $SS$, $BS$, $R_t$, $T_t$, $\hat{T_t}$. We take $SS$, $BS$ and $R_t$ as values shown in Tabel \ref{table:1}. $T_t$ and $\hat{T_t}$ are automatically calculated as 168 and 2. These values make up the baseline. When we test one of them, we keep the others the same as the baseline. The validation strategy is same as experiments in \S\ref{section:6.2}.

\noindent \textbf{Settings of \S\ref{section:6.5}.} In \S\ref{section:6.5}, we evaluate \textsc{threaTrace}'s runtime performance with varying parameters and compare with Unicorn and ProvDetector, using Unicorn SC-2 dataset. The parameters we evaluate are $SS$ and $BS$. We test one parameter and set the others as the baseline (Table \ref{table:1}). The runtime performance of Unicorn and ProvDetector are recorded during their execution in the same machine as \textsc{threaTrace}.

\noindent\textbf{Settings of \S\ref{section:a2}.} We study and evaluate the optimization-based evasion attack designed for \textsc{threaTrace} in \S\ref{section:a2.2} with Unicorn SC-2 dataset. The validation strategy is the same as experiments in \S\ref{section:6.2} and we first obtain anomalous nodes. After that, we solve the optimization function to gain the features of adversarial samples. The number of them is 100. Finally, we use the testing set, which contains the adversarial samples, for evaluation.

\noindent\textbf{Settings of \S\ref{section:a4}.} In \S\ref{section:a4}, we study and evaluate the overfitting problem for the stacked multi-model framework of \textsc{threaTrace}'s with Unicorn SC-2 dataset. We first conduct the same validation strategy as \S\ref{section:6.2} to split the training and testing set. Then, we split the training set as training set and validation set at a rate of 8:2. Finally, we vary the training set's proportion and number of training iterations for evaluation.

\noindent\textbf{Settings of \S\ref{section:a5}.} In \S\ref{section:a5}, we study and evaluate the data missing problem in the provenance graph with Unicorn SC-2 dataset. We conduct the same validation strategy as \S\ref{section:6.2} to split the training and testing set. After that, we randomly drop some data (edges) in training graphs and testing graphs to perform experiments.

\subsection{Evaluation Metrics}
\label{section:a3.3}

We introduce the definition of metrics we used for evaluating \textsc{threaTrace}, including \textbf{Precision/Recall/Accuracy/F-score and FPR/FNR}. \textsc{threaTrace} is a binary classification (benign or anomalous) tasks. Therefore, we first count the true positives (TP), true negatives (TN), false positives (FP), and false negatives (FN). After that, we can define the metrics mentioned above:

$Precision = \frac{TP}{TP + FP}, \quad Recall = \frac{TP}{TP + FN},$

~\\

$Accuracy = \frac{TP + TN}{TP + TN + FP + FN}, \text{F-score} = \frac{2 \times Precision \times Recall}{Precision + Recall},$

~\\

$FPR = \frac{FP}{FP + TN},\quad FNR = \frac{FN}{FN+TP}$

\begin{figure}[htbp]
\centerline{\includegraphics[width=0.5\textwidth]{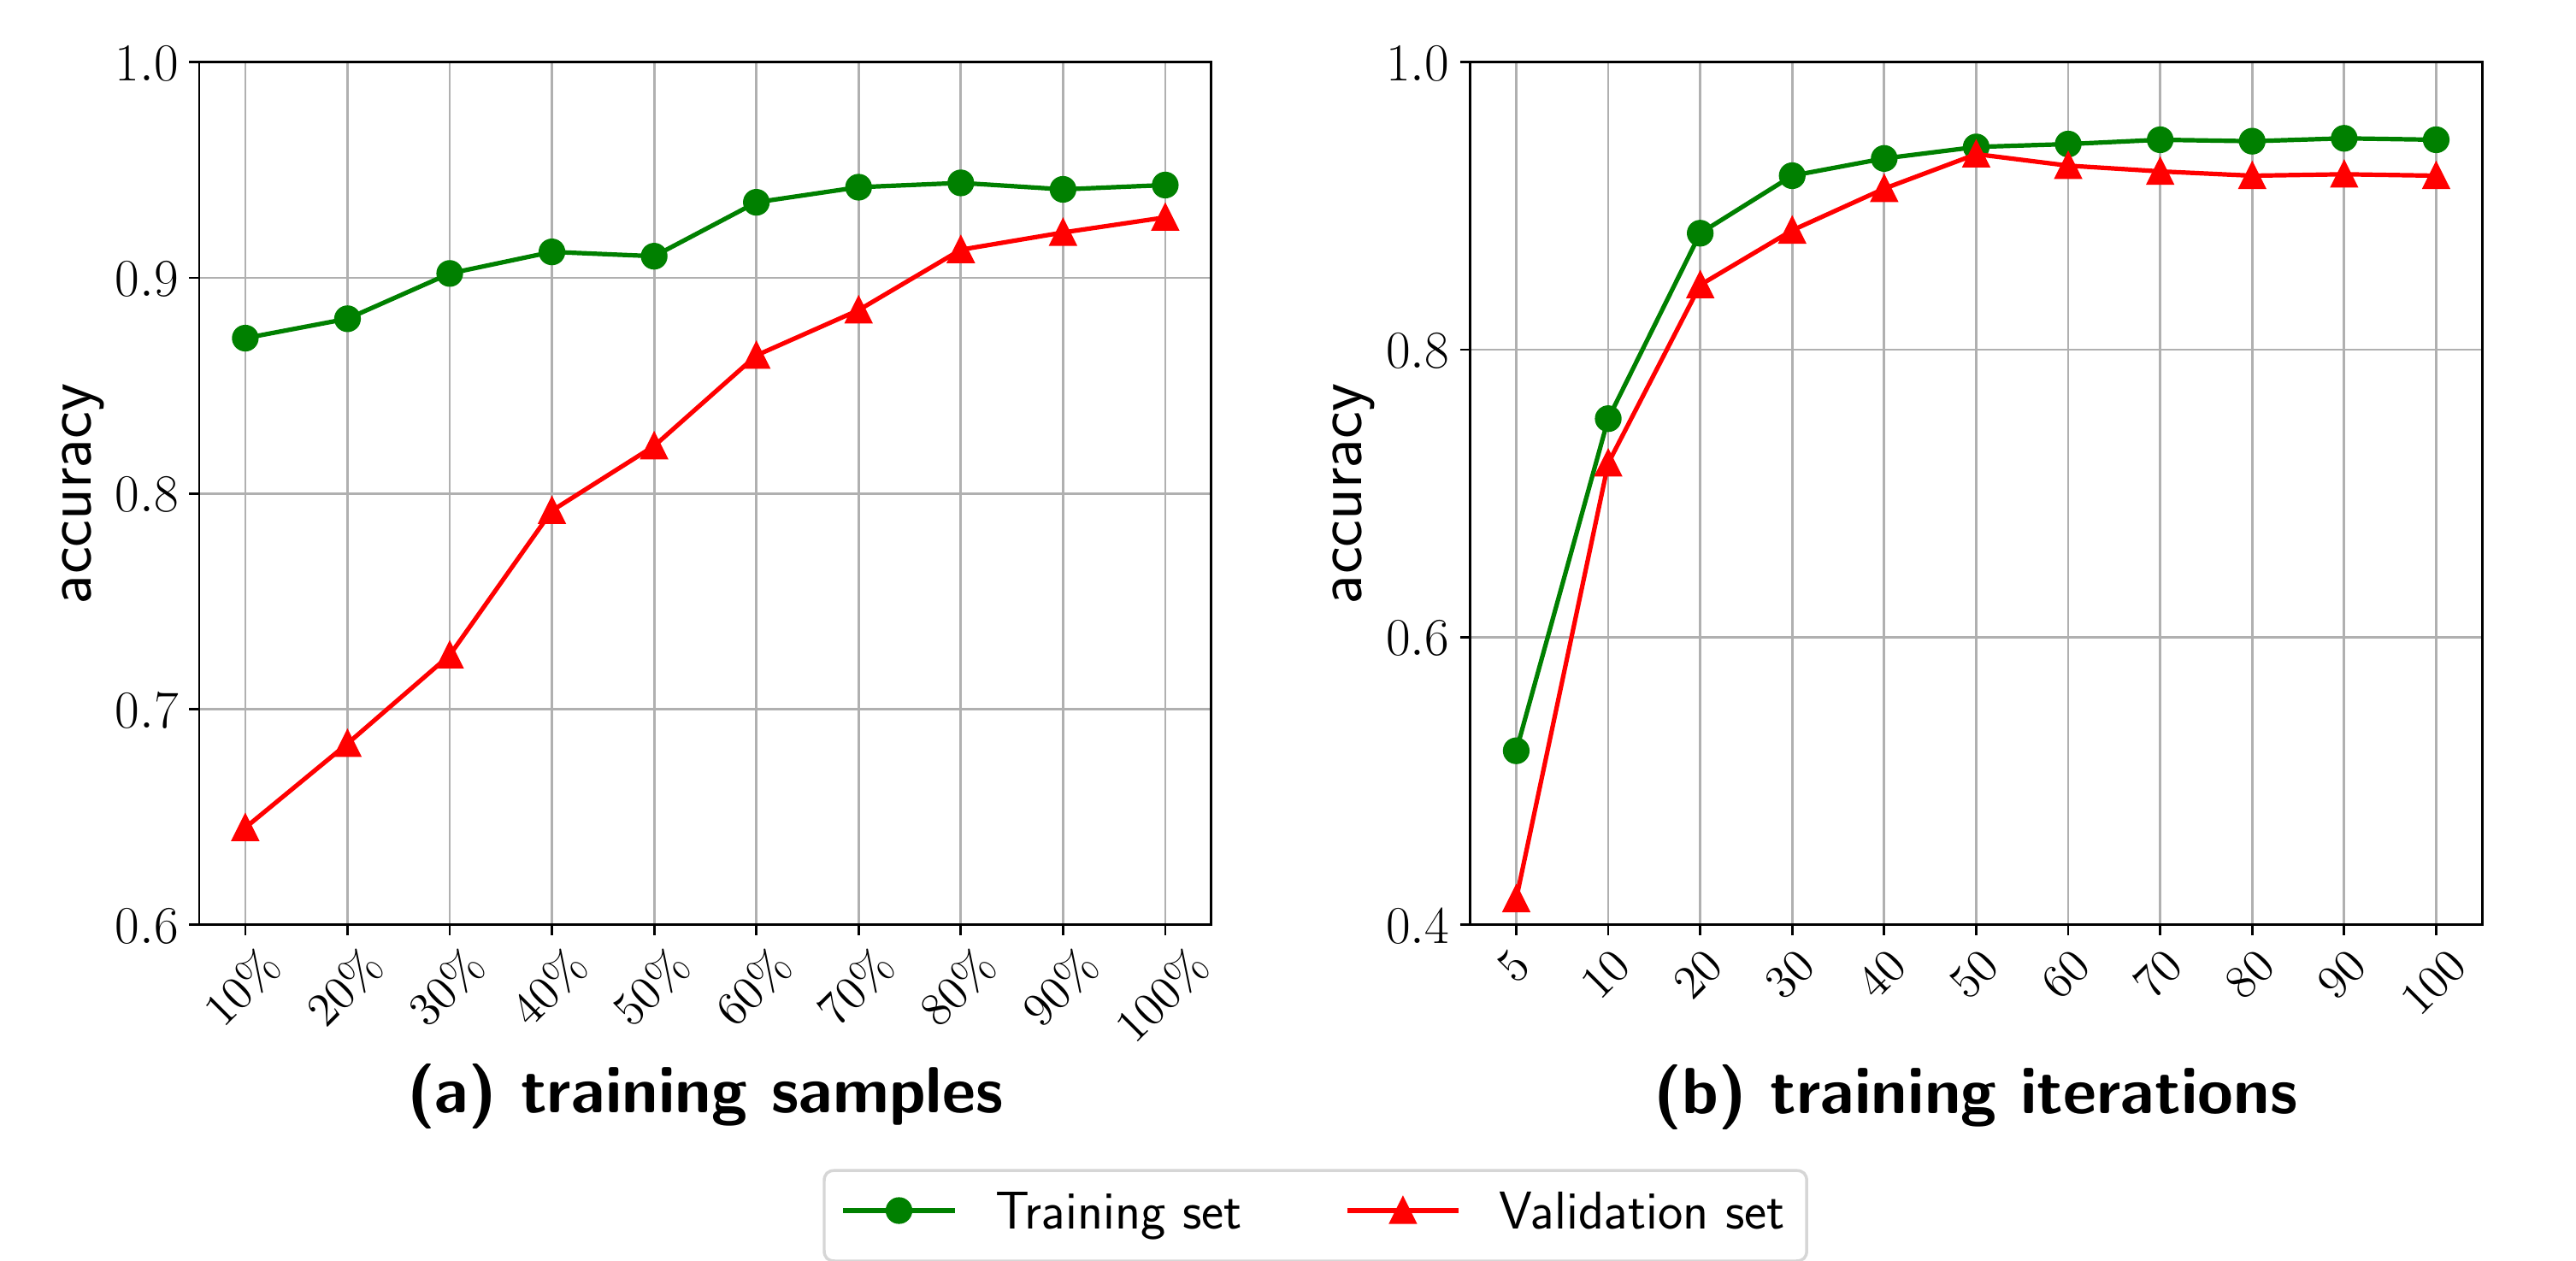}}
\caption{Learning curves.}
\label{fig:9}
\end{figure} 	

\begin{figure*}[htbp]
\centerline{\includegraphics[width=1.0\textwidth]{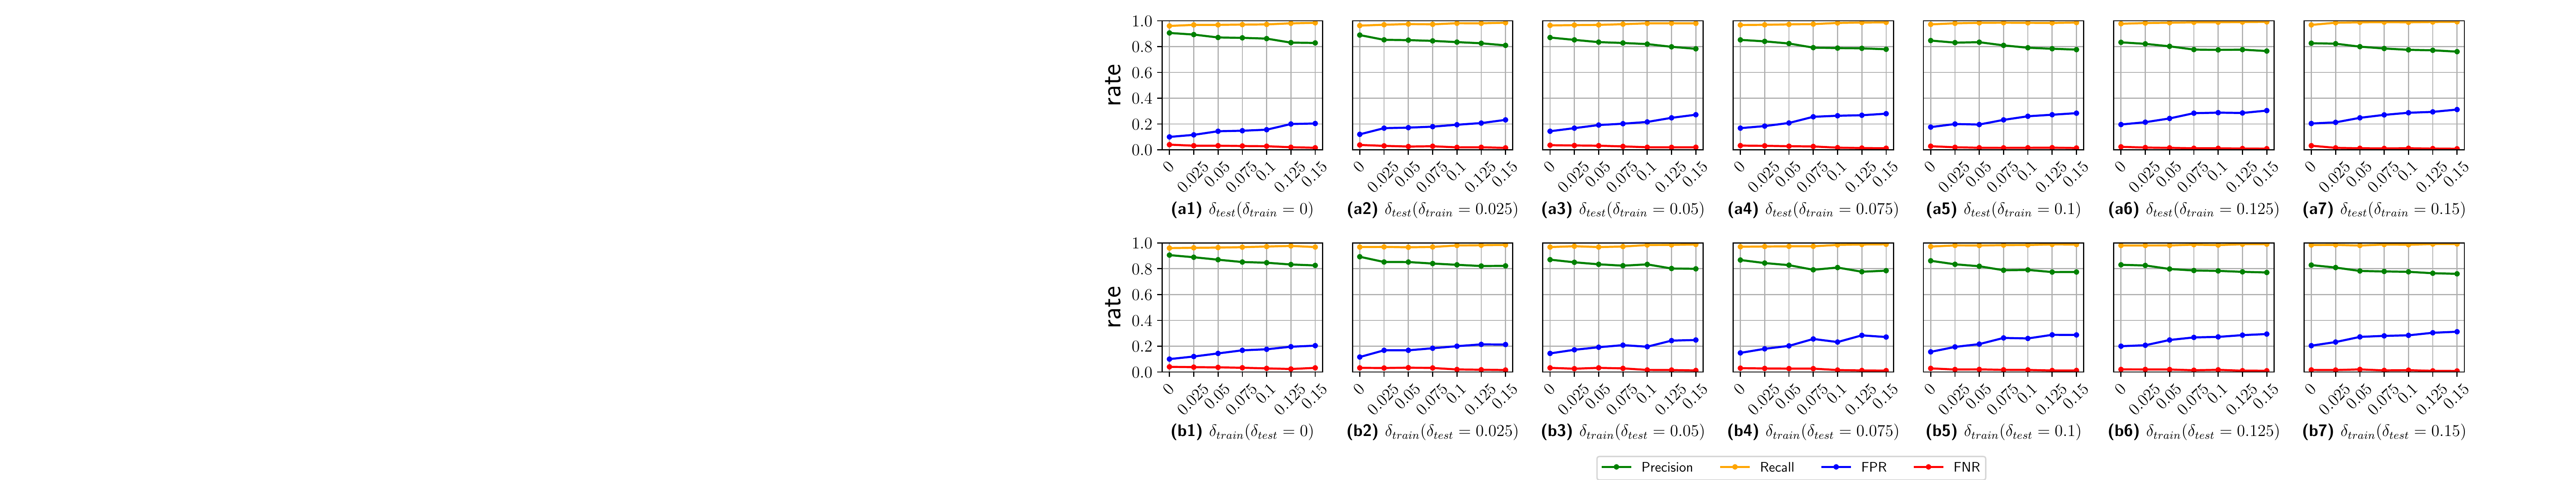}}
\caption{Results of data missing experiments.}
\label{fig:12}
\end{figure*}

\section{Overfitting problem}
\label{section:a4}

Below, we provide the discussion and evaluation of the overfitting problem in three aspects: What is overfitting? Does \textsc{threaTrace} have overfitting problem? How to solve overfitting?

\subsection{What is overfitting?}

\label{section:a4.1}

In a machine learning task, a model is \textit{overfitting} when it performs well in the training data while has a bad performance in validating data or testing data. It is typically because the model does not learn the general distribution after the training phase.

\subsection{Does \textsc{threaTrace} have overfitting problem?}
\label{section:a4.1}

A traditional method to observe whether the model is overfitting is analyzing the \textit{learning curve}. A learning curve plots the evaluation metric of a model for a training dataset and a validation dataset with the same parameters. It is useful to determine a model's different performance between a training dataset and a validation dataset in various x-axis values. The x-axis of a learning curve is either the number of training samples or iterations during training. As introduced in \S\ref{section:6}, \textsc{threaTrace} essentially solves a classification problem: the model learns different classes of benign nodes during the training phase and detects anomaly nodes based on the misclassification during the execution phase. Therefore, we use the training set of experiments in \S\ref{section:6.2} and split it as a training set and validation set at a rate of 8:2 to compare the performance between the classification results of training set and validation set. We explore the learning curve of \textsc{threaTrace} as shown in Figure \ref{fig:9}. The default values of training samples and iterations' numbers are 100\% and 60.

The results show that with the increasing of the training iterations' number, \textsc{threaTrace}'s accuracy in training set is increasing. In validation set, the accuracy increases first and turns down at a particular point. The problem of overfitting is least serious at that point. In the case of the number of training samples, the accuracy in the training set and validation set keep increasing together. From these two figures, we discover that with the default values of training samples and iterations' number (100\% and 60), the accuracy in training data is similar to that in validating data. Therefore, \textsc{threaTrace} does not have a severe overfitting problem. In the following subsection, we discuss some methods to avoid overfitting.

\subsection{How to solve overfitting?}
\label{section:a4.3}

We provide three approaches to avoid overfitting as follows.

\textbf{(1) Stop early.} A large number of iterations of training is one of the causes of overfitting. Therefore, stopping training as soon as possible can avoid overfitting to some extent.

\textbf{(2) More training data.} The results in Figure \ref{fig:9} show that more training data can help reduce the effect of overfitting.

\textbf{(3) Ensemble learning.} More models can prevent overfitting in a particular model. It can also explain why the multi-model framework of \textsc{threaTrace} does not have serious overfitting problems.

\section{Missing data}
\label{section:a5}

In this section, we evaluate how \textsc{threaTrace}'s detection performance is affected under the absence of data. The dataset we use is Unicorn SC-2 dataset. We set parameters $\delta_{train}$ and $\delta_{test}$, which mean the data loss proportion of training data and testing data. We randomly delete training data and testing data based on $\delta_{train}$ and $\delta_{test}$. We evaluate different $\delta_{train}$ of training data and $\delta_{test}$ of testing data. The results are shown in Figure \ref{fig:12}.

As the results shown, missing data in training set and testing data will affect the detection performance. As the data loss rate increases, the FPR increases and Precision decreases. When data missing happens in training set, the model cannot learn information of benign nodes adequately, which thus results in more FPs. Note that insufficiently learning of benign data decreases FNR and increases Recall because abnormal samples are more likely to deviate from what the model has learned. When data missing happens in testing set, both benign nodes and abnormal nodes tend to be detected as abnormal, which thus results in higher Recall/FPR and lower Precision/FNR. In this paper, we use external tools for data collection. Fortunately, these tools are reliable to capture the entire data provenance in a system \S\ref{section:7}. Therefore, data missing problems may rarely occur in practice.
